# Supplementary material for: Strain-Tunable GaAs Quantum dot: A Nearly Dephasing-Free Source of Entangled Photon Pairs on Demand
Source: arXiv:1801.06655 ancillary file (2018-10-10)
Supplement: Supplementary file 1 [file Supplementary_Materials_for_Strain_tunable_GaAs_quantum_dot__a_nearly_dephasing_free_source_of_entangled_photon_pairs_on_demand.pdf]

# Supplementary Materials for Strain-Tunable GaAs Quantum dot: A Nearly Dephasing-Free Source of Entangled Photon Pairs on Demand

Daniel Huber,[1,*] Marcus Reindl,[1,†] Saimon Filipe Covre da Silva,[1,†] Christian Schimpf,[1] Javier Martín-Sánchez,[1,2] Huiying Huang,[1] Giovanni Piredda,[3] Johannes Edlinger,[3] Armando Rastelli,[1,‡] and Rinaldo Trotta[1,4,§]

[1]*Institute of Semiconductor and Solid State Physics, Johannes Kepler University, Linz, Altenbergerstrae 69, 4040, Austria*

[2]*Department of Physics, University of Oviedo, 33007 Oviedo, Spain*

[3]*Forschungszentrum Mikrotechnik, FH Vorarlberg, Hochschulstrae 1, A-6850 Dornbirn, Austria*

[4]*Department of Physics, Sapienza University of Rome, Piazzale Aldo Moro 5, 00185 Rome, Italy*

**CONTENTS**

I. Methods 2
A. Device Fabrication 2
B. Measurement Setup 3
II. Measurement of the entanglement fidelity with a reduced measurement set on QD1 4
III. Effect of the waveplate retardence 6
IV. Polarization resolved $g^{(2)}$ measurements on QD2 7
V. Fidelity of a rotated state 8
VI. Entanglement background light correction 9
References 11

# I. METHODS

## A. Device Fabrication

For this study, highly symmetric GaAs quantum dots, grown by solid state molecular beam epitaxy via the droplet etching method, are used. In particular, a GaAs substrate is overgrown with a 332 nm buffer layer, on which 9 pairs of alternating $Al_{0.95}Ga_{0.05}As/Al_{0.2}Ga_{0.8}As$ layers with a thickness of 67 nm and 58 nm, respectively, are deposited. On top of this layer structure, which forms the back mirror of a planar cavity, a single 20 nm $Al_{0.2}Ga_{0.8}As$ layer followed by a 63 nm thick $Ga_{0.6}Al_{0.4}As$ layer is grown. The latter layer is hosting the nanoholes, which are fabricated using aluminum droplet etching. The QDs are then obtained by depositing 2 nm of GaAs that fills the nanoholes, which are subsequently overgrown with a 58 nm $Ga_{0.6}Al_{0.4}As$ layer, acting as a top barrier and a single 20 nm $Al_{0.2}Ga_{0.8}As$ layer. Finally, two pairs of $Al_{0.95}Ga_{0.05}As/Al_{0.2}Ga_{0.8}As$ layers were grown as distributed Bragg reflector to complete the cavity.

For the device fabrication (see Fig. 1), a 2x2 mm sample piece is thinned down to a thickness of 30 $\mu$m via mechanical lapping. The resulting membrane is bonded on a

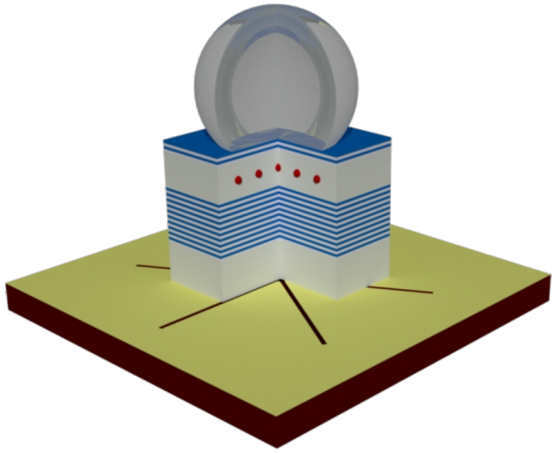

FIG. 1. **Sketch of the device structure.** On top of the structure a solid immersion lens is placed. The QDs (red spheres) are embedded in a planar cavity with distributed Bragg reflector mirrors. The sample is bonded onto a piezo electric actuator (golden part) similar to the one used in Ref.[1,2].

micromachined 300-mm-thick $[Pb(Mg_{1/3}Nb_{2/3})O_3]_{0.72}$-$[PbTiO_3]_{0.28}$ (PMN-PT) piezoelectric substrate by epoxy photoresist (see Ref.[3]). Finally, on top of the membrane, a hemispherical solid immersion lens, made of zirconia, is placed. Differently from previous works that use thin nanomembrane (thickness of 100 nm)[1,2], the micromachined PMN-PT used here hosts a relatively thick membrane with a 2 mm thick SIL on its top surface. The proper operation of this device implies that arbitrary strain-fields can be used to suppress the fine-structure splitting of QDs embedded in other thick photonic structures (even with large aspect ratio) capable of boosting the flux of QD photons[4,5].

### B. Measurement Setup

The measurements are performed at a sample temperature of 5 K in a helium-flow cryostat. The quantum dots are resonantly pumped by a titanium sapphire femtosecond laser featuring a bandwidth of 100 fs and a repetition rate of 80 MHz, which is shaped into 9 ps pulses by a 4f-pulse-shaper setup. The excitation laser is focused via an objective with a numerical aperture of 0.42. For the time resolved measurements the emitted exciton and biexciton photons are spectrally separated using two tunable notch filters with a full width

at half maximum of 400 $\mu$eV. Here, the first filter is reflecting the exciton photons under a defined angle while the other wavelengths are transmitted. The second notch is used to select the XX photons in the same way. The exciton and biexciton photons are guided into single mode fibers, respectively, which are connected to avalanche photodiode detectors with a timing resolution of about 500 ps. In front of each fiber coupler polarization optics consisting of an achromatic lambda/2-, lambda/4 (Thorlabs) waveplate and a linear polarizer are placed to perform polarization resolved cross-correlation measurements. For the decay time measurements a detector with about 100 ps timing resolution is used. The fine structure measurements are performed using a spectrometer equipped with a 1800 grooves/mm grating. Using Lorentzian fitting of both the exciton and biexciton lines, the FSS can be measured with sub $\mu$eV resolution.

## II. MEASUREMENT OF THE ENTANGLEMENT FIDELITY WITH A REDUCED MEASUREMENT SET ON QD1

We calculated the fidelity via a reduce measurement set of six according to

$$f = \frac{1 + C_{\text{linear}} + C_{\text{diagonal}} - C_{\text{circular}}}{4}, \tag{1}$$

where $C$ are the correlations visibilities according to

$$C_{\mu} = \frac{g^2_{XX,X} - g^2_{XX,\overline{X}}}{g^2_{XX,X} + g^2_{XX,\overline{X}}}, \tag{2}$$

where where $g^2_{XX,X}$ and $g^2_{XX,\overline{X}}$ is the co- and the cross-polarized correlation measurement, respectively, in the basis $\mu$. The cross correlation measurements for vertical (horizontal), diagonal (antidiagonal) and circularly right (circularly left) polarized photons are shown in Fig.2.

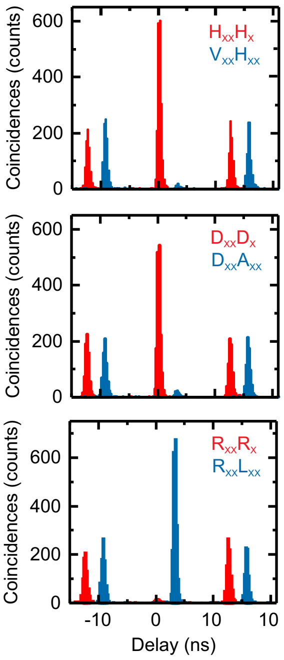


FIG. 2. **Measurement of the entanglement fidelity with a reduced measurement set on QD1.** Cross-correlation between biexciton (XX) and exciton (X) photons. $V_{XX,X}$ ($H_{XX,X}$), $D_{XX,X}$ ($A_{XX,X}$) and $R_{XX,X}$ ($L_{XX,X}$) indicate vertical (horizontal), diagonal (antidiagonal) and circularly right (circularly left) polarized photons. The graphs for copolarized (red) and cross-polarized (blue) photons are temporally shifted by 3 ns for clarity.

## III. EFFECT OF THE WAVEPLATE RETARDENCE

We calculated the effect of the waveplate retardance on the fidelity and concurrence on the basis of the measurement data of QD1 by varying the retardance of the lambda/2 and lambda /4 around their target values (see Fig.3). The result shows maxima far off the taget values. However, we point out that one can not simply use the maximum value as result, as the relation between measurement data and resulting density matrix is not unique. In other words, the retardance of the used waveplates has to be known.

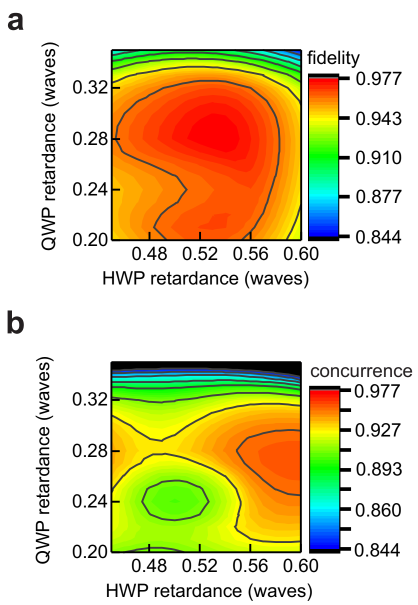


FIG. 3. **Effect of the waveplate retardance onto the measured degree of entanglement.** (a) Entanglement fidelity and (b) concurrence versus the half-waveplate (HWP) and quarter-waveplate (QWP) retardance.

## IV. POLARIZATION RESOLVED $g^{(2)}$ MEASUREMENTS ON QD2

| measurement | $g^{(2)}(0)$ |
|---|---|
| $X_H$ | 0.009(3) |
| $X_V$ | 0.025(5) |
| $X_D$ | 0.017(4) |
| $X_A$ | 0.010(3) |
| $X_R$ | 0.015(3) |
| $X_L$ | 0.010(4) |
| $XX_H$ | 0.003(2) |
| $XX_V$ | 0.036(7) |
| $XX_D$ | 0.012(3) |
| $XX_A$ | 0.014(4) |
| $XX_R$ | 0.015(4) |
| $XX_L$ | 0.021(5) |

TABLE I. **Polarization-dependent auto correlation measurements.** The table shows the values of the secondary auto correlation function at zero time delay ($g^2(0)$) for biexciton (XX) and exciton (X) for linear horizontal (H), vertical (V), diagonal (D) and antidiagonal (A) as well as circular right (R) and left (L) polarized photons.

## V. FIDELITY OF A ROTATED STATE

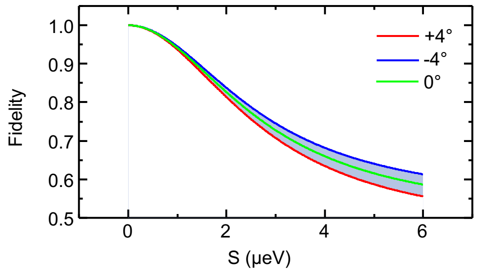


FIG. 4. **Fidelity of a rotated state.** The plot shows the deviation between the unrotated ($\omega = 0°$) entangled state (see green curve) and a rotation up to $\omega = \pm 4°$ (see red and blue curve, respectively). The fidelity calculated out of the density matrix is robust against such a rotation.

The calculation of the fidelity with Eq. 2 from the main paper via a reduced set of only 6 correlation measurements can cover the true value of the fidelity if the fine structure splitting $S \neq 0$ and an additional static phase $\omega$ introduced by the setup rotates the state (see Fig.4). Therefore the entangled state (see Eq. 1 in the main paper) can be written as $|\psi\rangle = U(\omega) \cdot 1/\sqrt{2}(|H_{\rm XX}\rangle\,|H_{\rm X}\rangle + e^{\frac{iSt}{\hbar}}\,|V_{\rm XX}\rangle\,|V_{\rm X}\rangle)$, where U is a rotation matrix as a function of $\omega$.

## VI. ENTANGLEMENT BACKGROUND LIGHT CORRECTION

In the following we derive a statistical model to estimate the influence of the background onto a polarization resolved cross-correlation measurement between exciton and biexciton. Therefore we assume a photon pair extraction efficiency $<< 1$. Further, to increase the readability we do not handle the detection and transmission efficiencies of the setup during the calculation as their contributions cancel.

The probability to create an exciton or a background photon and transmit it through a polarizer in the eigenstate $i$ within the spectral range of the exciton notch filter is given by:

$$p_{x,i} = a_x t_{x,i} \tag{3}$$

and

$$p_{bx,i} = a_{bx} t_{bx,i}, \tag{4}$$

respectively. Here $a_{x(bx)}$ is the generation probability of an exciton ( one or more photons background) photon(s) within a time bin considered in the $g^2(t)$ and $t_{x(xb),i}$ its probability to be transmitted through the analyzer state $i$.

In a Hanbury-Brown-Twiss like experiment in start-stop mode the $g^{(2)}(t)$ - autocorrelation function at $t = 0$ is given by

$$g^{(2)}(0) = N(c_{x,i} + p_{x,i}p_{bx,i} + p_{bx,i}p_{bx,i}), \tag{5}$$

where $N$ is a constant and $c_{x,i}$ is the probability to get an coincidence by two emitted exciton photons. Hereby, we assume that $c_{x,i} = 0$ as the exciton transition emits only single photons[6]. Inserting Eq. 3 and Eq. 4 in Eq. 5 yields:

$$g^{(2)}(0) = N(a_x t_{x,i} a_{bx} t_{bx,i} + a_{bx}^2 t_{bx,i}^2) \tag{6}$$

In the same way the first side peak of the $g^2$-function can be calculated to

$$\begin{aligned} g^{(2)}(\tau) &= N(p_{x,i}(0)p_{x,i}(\tau) + p_{x,i}(0)p_{bx,i}(\tau) + p_{x,i}(\tau)p_{bx,i}(0) \\ &\quad + p_{bx,i}(0)p_{bx,i}(\tau)) \\ &= N(a_x^2 t_{x,i}^2 + a_{bx}^2 t_{bx,i}^2 + 2a_x t_{x,i} a_{bx} t_{bx,i}) \end{aligned} \tag{7}$$

assuming that $p_{x,i}$ is constant over time. Due to the low background photon generation rate $a_{bx}$, the ratio between $g^{(2)}(0)$ and $g^{(2)}(\tau)$ can be expanded in a Taylor series around $a_{bx} = 0$, which leads to

$$\frac{g^2(0)}{g^2(\tau)} = \frac{a_{bx}t_{bx,i}}{a_{bx}t_{bx,i} + a_x t_{x,i}} \approx \frac{a_{bx}t_{bx,i}}{a_x t_{x,i}} - \frac{t_{bx,i}^2 a_{bx}^2}{a_x^2 t_{x,i}^2} + O[a_{bx}]^3. \tag{8}$$

By taking to account that $a_x \approx 1$ in $\pi-$pulse and $a_{bx} << a_x$ we can safely neglect the quadratic and other higher order terms. Further, $t_{x,i} = \frac{1}{2}$, if we assume two modes $i = \{H, V\}$ for an unpolarized QD source and thus Eq. 8 simplifies to

$$g^{(2)}_{X,i} = \frac{g^2(0)}{g^2(\tau)} = 2 \cdot t_{bx,i} a_{bx}. \tag{9}$$

For the biexciton a similar expression can be derived:

$$g^{(2)}_{XX,i} = 2 \cdot t_{bxx,i} a_{bxx}. \tag{10}$$

This allows us to estimate the amount of time correlated background emission by measuring the $g^2(t)$- autocorrelation function for exciton and biexciton separately in all 6 polarization basis.

To correct the raw data for the background emission we have to calculate the probability $b_{ik}$ to get a coincidence related to a background photon in the polarization passing a analyzer in the eigenstate state $i$,$k$. It follows that

$$b_{ik} = \frac{a_{xx}t_{xx,i}g^{(2)}_{X,k}}{2} + \frac{a_x t_{x,k} g^{(2)}_{XX,i}}{2} + \frac{g^{(2)}_{XX,i} g^{(2)}_{X,k}}{4} \tag{11}$$

with $a_{xx}t_{xx,i} = a_x t_{x,k} \approx \frac{1}{2}$ and $g^{(2)}_{XX,i} g^{(2)}_{X,k} \approx 0$ this equation simplifies into

$$b_{ik} = \frac{1}{4}(g^{(2)}_{X,k} + g^{(2)}_{XX,i}). \tag{12}$$

The number of coincidences in the central peak of a cross-correlation measurement in the basis $i, k$ is then given by

$$\begin{aligned} n_{c,ik} = \widetilde{N}(4 \langle i,k| \rho |i,k\rangle\, g^{(2)}_{X,XX} + \\ b_{i,k} g^{(2)}_b + R g^{(2)}_R) \end{aligned} \tag{13}$$

where $\widetilde{N}$ is a constant, $\rho$ is the two-photon density matrix of the entangled state, $g^{(2)}_{X,XX}$, $g^{(2)}_{b}$ and $g^{(2)}_{R}$ are the values of the cross-correlation function between unpolarized exciton and biexciton photons, exciton and biexciton background photons and non entangled exciton and biexciton photons at $\tau$=0, respectively and $R$ is the probability to generate a non entangled photon pair not related to background. As the background is due to coherent laser light it follows that $g^{(2)}_{b} = 1$. Furthermore we assume that $g^{(2)}_{R} \approx g^{(2)}_{X,XX}$.

The number of coincidences in a side peak instead is given by

$$n_{s,ik} = \widetilde{N}(1/2 + b_{i,k} + R). \tag{14}$$

The relation

$$\frac{n_{c,ik}}{n_{s,ik}} = \frac{p_e + b_{ik} + R}{\frac{1}{2} + b_{ik} + R}, \tag{15}$$

where $p_e$ is the probability to have a coincidence from an entangled photon pair, allows us to get an estimate for $R$ and to calculate $\frac{n_{c,ik}}{n_{s,ik}}$ without background to

$$\frac{n'_{c,ik}}{n'_{s,ik}} = \frac{p_e + R}{\frac{1}{2} + R}. \tag{16}$$

This result can be used to calculate the background corrected density matrix according to the formalism presented in Ref.[7].

---


* daniel.huber@jku.at

† These two authors contributed equally

‡ armando.rastelli@jku.at

§ rinaldo.trotta@uniroma1.it



1 R. Trotta, J. Martín-Sánchez, C. Schimpf, E. Zallo, S. Stroj, J. Edlinger, and A. Rastelli, Nature Communications **7**, 10375 (2016).

2 J. Martín-Sánchez, R. Trotta, G. Piredda, C. Schimpf, G. Trevisi, L. Seravalli, P. Frigeri, S. Stroj, T. Lettner, M. Reindl, J. S. Wildmann, J. Edlinger, and A. Rastelli, Advanced Optical Materials **4**, 682 (2016).

[3] D. Ziss, J. Martín-Sánchez, T. Lettner, A. Halilovic, G. Trevisi, R. Trotta, A. Rastelli, and J. Stangl, Journal of Applied Physics **121**, 1 (2017).

[4] N. Somaschi, V. Giesz, L. De Santis, J. C. Loredo, M. P. Almeida, G. Hornecker, S. L. Portalupi, S. L. Portalupi, T. Grange, C. Antn, J. Demory, C. Gmez, I. Sagnes, N. D. Lanzillotti-Kimura, A. Lematre, A. Auffeves, A. G. White, L. Lanco, and P. Senellart, Nature Photonics **10**, 340 (2016).

[5] X. Ding, Y. He, Z.-C. Duan, N. Gregersen, M.-C. Chen, S. Unsleber, S. Maier, C. Schneider, M. Kamp, S. Höfling, C.-Y. Lu, and J.-W. Pan, Phys. Rev. Lett. **116**, 020401 (2016).

[6] L. Schweickert, K. D. Jöns, K. D. Zeuner, S. F. C. da Silva, H. Huang, T. Lettner, M. Reindl, J. Zichi, R. Trotta, A. Rastelli, and V. Zwiller, Appl. Phys. Lett. **112**, 093106 (2018).

[7] D. F. V. James, P. G. Kwiat, W. J. Munro, and A. G. White, Phys. Rev. A **64**, 052312 (2001).
